# Supplementary material for: Predictability and Comprehensibility in Post-Hoc XAI Methods: A User-Centered Analysis
Source: arXiv:2309.11987 source file (2023-09-21)
Supplement: Supplementary file 1 [file appendix.tex]

\section{Pre-test Survey}
\label{Pre_Test_Survey}

We presented users with 10 Data Science know-How questions. The following, lists the questions of our pre-test survey:
\begin{enumerate}
    \item Which of the following terms are correct? (Please choose one)
    \begin{itemize}
        \item Artificial Intelligence = Deep Learning = Machine Learning 
        \item (Machine Learning = Deep Learning) < Artificial Intelligence  
        \item Artificial Intelligence < Machine learning < Deep Learning  
        \item Artificial Intelligence > Machine learning > Deep Learning  
        \item I do not know 
    \end{itemize}
    
    \item  Which figure depicts a normal distribution? We presented the participants with 4 different distributions: uniform, Poisson, Gama and normal distributions.
    
    \item What are the equations of a linear and logistic regression? (You may select more than one box). 
    
    \item Which of the following statements are correct for supervised vs unsupervised learning? (You may select one or more boxes)
\begin{itemize}
        \item Clustering algorithms are the popular approach for supervised learning.
        \item Clustering algorithms are the popular approach for unsupervised learning.
        \item Clustering algorithms are the popular approach for semi-supervised learning
        \item I do not know
    \end{itemize}        

    \item How is the recall (sensitivity) metric calculated?
    
    \item  What value would you choose for k in your k-means clustering w.r.t. the figure below?

    \item The figure below depicts the box-plot of four employee groups' decision scores on their work environment quality survey. Please answer the following questions.
    \begin{itemize}
        \item  What does the black line in the middle of the box-plots indicate?
        \item  Looking at the bar plots above, which group has a high level of agreement on the work environment quality?
        \item  Looking at the bar plots above, which group has quite a low level of agreement with each other?
        \item  Looking at the bar plots above, which group significantly disagrees with the other groups?
    \end{itemize}

    \item Difference between a validation set and Test is that ...
        \begin{itemize}
            \item  A test set is used while the model is in a training phase to tune the model's parameter, a validation set is a set where the tuned model is evaluated with.
            \item  A test set should contain some or all the data from the train set.  agreement on the work environment quality?
            \item  A validation set is used while the model is in a training phase to tune the model's parameter, a test set is a set where A validation set is used while the model is in a training phase to tune the model's parameter, a test set is a set where the tuned model is evaluated with.
            \item  A validation set should contain some or all the data from the train set.
            \item I do not know
    \end{itemize}
    
    \item Three different machine learning models were trained to hit the center and the following figures depict the estimations of these models.
        \begin{itemize}
            \item  Model 1 ( We demonstrated the model with a figure of a dart board, which the dart where concentrated at a point further away from the center. This indicates a model with high bias.) 
            \item  Model 2 ( We demonstrated the model with a figure of a dart board, which the dart where randomly distributed over the area of the board. This indicates a model with high variance.) 
            \item  Model 3 ( We demonstrated the model with a figure of a dart board, which the dart where very close to each other, and to the center. This indicates a model with a trade-off between variance and bias.) 
            \item I do not know
    \end{itemize}    

\end{enumerate}

\section{Comprehensibility}
\label{app:coding_rules}

%Figure~\ref{fig:} depicts one of two tasks of assignment one for measuring the comprehensibility. The explanations are the output of LIME

%    \begin{figure}[h]
%        \centering
%        \caption{Task 1 () of the survey contains 3 explanations of three different samples %from the same class. Each sample itself is represented by a bar-plot, and above the bar-plots, we present the participants with the actual label of the samples, as well as the predicted samples. At the bottom of the Figure, the test sample is presented, which we asked the participants to draw conclusions and answer the questions.}
%        \includegraphics[width=\linewidth]{figures/assignmen_.png}
%        \label{fig:}
%    \end{figure}

We qualitatively analized our participants' feedback, and coded our transcribed interviews, following the Mayring inductive qualitative analysis structure \cite{mayring2004qualitative}, into the following three categories:

\begin{itemize}
    \item C1: C1 more difficult than C2
    \begin{itemize}
        \item Definition: High subjective conviction to have answered the  questions with more mental demand than C2 questions, which means:
        i) to be clear about the task’s difficulty and the responses to the tasks, ii) to have a negative feeling about the correctness of their answers compared to C2 questions.

        \item Example: “I find  more difficult than C2. I was not very familiar with using the visualizations, the samples and what the features represent, how they correlate. These things were already more clear to me when I was answering C2 questions. I already knew how to use the visualizations to find the answers for C2. I still answered correctly for both I think, but needed longer to find the answers for ” (UID=27).
        \item Coding Rule: All the aspects of the definition has to point to “ more difficult”. No aspect only “ and C2 equally difficult”. Otherwise C3 -  and C2 equally difficult
    \end{itemize}
    
    \item C2: C2 more difficult than 
    \begin{itemize}
        \item Definition: Conviction to have badly coped with answering the question of C2, which means not to know where to find the information that can guide the user to the correct answer, and to have a negative, pessimistic feeling in answering the questions.

        \item Example: “I found C2 more difficult than . The explanations were more or less intuitive to understand, but for example, the range for one of the features was not well presented in the explanations and why its effects are changing. That was confusing for me to answer the C2 questions.” (UID=31) 
        
        \item Coding Rule: All two aspects of definition point to how difficult C2 was for the user, no fluctuations recognizable
    \end{itemize}
    
    \item C3:  and C2 equally difficult
    \begin{itemize}
        \item Definition: Only partly or fluctuating conviction to have confidently answered to the questions
        \item Example: “Difficult to say, I found them both difficult to answer. I didn't get exactly how to use the explanations to answer the questions. Specially for the features that were asked whether they decrease the  probability of the class. There was no visible information to know this. ” (UID=33)
        \item Coding Rule: If not all aspects of definition point to " more difficult" or "C2 more difficult"
    \end{itemize}
\end{itemize}

%\section{Trust}
%\label{Appx_Trust}

%Figure~\ref{fig:T4_SHAP} depicts one of two tasks of assignment two for measuring the trust using LIME explanations. The explanations are the output of SHAP.

%    \begin{figure}[h]
%        \centering
%            \caption{Task 4 (T4) of the survey contains 3 explanations of three different samples from the each class. Each sample itself is represented by a bar-plot, and above the bar-plots, we present the participants with the actual label of the samples, as well as the predicted samples. At the bottom of the Figure, the test sample is presented, which we asked the participants to draw conclusions and answer the questions.}
%        \includegraphics[width=\linewidth]{figures/assignmenC2_T4s.png}
%        \label{fig:T4_SHAP}
%    \end{figure}

\section{Users' Self-Confidence}
\label{Appx_RQ3_confidence}
We code our transcribed interviews for user's confidence, following the same instructions as before, into the following three categories:
For a high self-confidence category, the feedback must have:
\begin{itemize}
    \item positive modals – always, mostly, often, more often, very following the words confident or sure.
    \item positive verb – if (No or Not in the feedback) then it is a negative verb otherwise, positive verb.
    \item adjective: high, pretty, pretty much, overall, more or less, over/about x\% (where x> 66) following the words confident or sure.
\end{itemize}

For coding rules for low self-confidence, the feedback must have:
\begin{itemize}
    \item Negative modals – never, mostly, often, more often, very unsure. These (except never) should come with unsure
    \item Negative verb – if (No or Not in the feedback) then it is a negative verb otherwise, positive verb
    \item adjective: pretty, pretty much, overall, less than/about x\% following the words low confident or unsure (where x< 33)
\end{itemize}
We assign the user's feedback to the average self-confidence when it cannot be high or low self-confidence.

\section{User's Feedback}
\label{Appx_RQ3_feedback}
To categorize user's feedback as very helpful, we use the same qualitative encoding procedure. the feedback are categorized as follow:

\begin{itemize}
    \item H1: Very helpful to answer the test sample
    \begin{itemize}
        \item Definition: Similar to the high self-confidence category, high subjective feeling of having met the challenge well
        \item Example: "The visualizations helped to understand which features are often the main contributors and how the model orders the importance of the features based on their values," UID=0
        \item Coding Rule: All the aspects of the definition must point in the direction of "very helpful", at least no aspect should allow the diagnosis of more or less helpfulness; otherwise encoding for H2
    \end{itemize}
    
    \item H2: Only helpful to understand the explained samples
    \begin{itemize}
        \item Definition: Similar to the average self-confidence category, only understood the explained samples but could not apply the information to the new test sample.
        \item Example: "More or less it could help to understand the clear distinctions between explained samples from different classes. But not enough to assume something for the test sample.", UID=1
        \item Coding Rule: If not all three aspects point to H1 or H3
    \end{itemize}
    
    \item H3: Note Helpful at all
    \begin{itemize}
        \item Definition: Similar to low self-confidence, the conviction of having poorly coped with the challenge
        \item Example: "I didn't get any insight using the visualizations, the visualizations were very confusing to me, and I couldn't make sense of the inequality ranges."
        \item Coding Rule: All aspects point to no helpfulness, otherwise encoding for H2.
    \end{itemize}
\end{itemize}
