# Supplementary material for: Predictability and Comprehensibility in Post-Hoc XAI Methods: A User-Centered Analysis
Source: arXiv:2309.11987 source file (2023-09-21)
Supplement: Supplementary file 2 [file Appendix.tex]

\appendix
\section{Appendix}
In table~\ref{table:sota}, we summarize the previous user studies, which evaluated model interpretations and explanations techniques. 

\begin{table}[h]
    \centering
    \caption{A summary of the existing studies for evaluating XAI approaches.}
    \label{table:sota}
     \scalebox{0.46}{
    \begin{tabular}{cccccccc}
        \toprule
        &&\multicolumn{2}{c}{Evaluation}&\multicolumn{4}{c}{Explanations}\\
        \cmidrule{2-8}
        Paper&Metric&Approach&Data&\multicolumn{2}{c}{Manipulated}&\multicolumn{2}{c}{Show}\\
        \cmidrule{5-8}
        &&&&Model&Examples&Preds&Labels\\
        \midrule

        %Alqaraawi et al.
        ~\cite{alqaraawi2020evaluating}&Compreh.&Quan.&Image&\xmark&\xmark&\cmark&\xmark\\
        \midrule

        %Hase et al.
        ~\cite{hase2020evaluating}&Simulation&Quan.&Text&\xmark&\cmark&\cmark&\xmark\\
                                             &(Trust)&&&&&\\
        % This work is also measures model behaviour prediction using explanations, but they don't call it trust ... they call it simulation ...
        \midrule

        %Kaur et al.
        ~\cite{kaur2020interpreting}&Trust&Quan.&Tabular&\xmark&\xmark&\cmark&\xmark\\
                                               &&Qual.&&&&\\
        \midrule
        
        %Lakkaraju et al.
        ~\cite{lakkaraju2020fool}&Trust&Quan.&Tabular&\cmark&\cmark&\xmark&\xmark\\
        \midrule
        
        %Mohseni et al.
        ~\cite{mohseni2018human}&Trust&Quan.&Image&\xmark&\xmark&\cmark&\xmark\\
                                 &&&Text&&&\\
        \midrule
        
        %Nourani et al.
        ~\cite{nourani2019effects}&Trust&Quan.&Image&\xmark&\cmark&\xmark&\xmark\\
        \midrule
        
        %Papenmeier et al.
        ~\cite{papenmeier2019model}&Trust&Quan.&Text&\xmark&\cmark&\xmark&\xmark\\
                                   &Compreh.&&&&&\\
        \midrule
        %Ribeiro et al.
        ~\cite{ribeiro2016should}&Trust&Quan.&Image&\cmark&\xmark&\cmark&\xmark\\
                                 &Compreh.&&Text&&&\\
        \midrule
        %Ribeiro et al.
        ~\cite{ribeiro2018anchors}&Compreh.&Quan.&Image&\xmark&\xmark&\cmark&\xmark\\
        
        \midrule
        %Schmidt et al.
        ~\cite{schmidt2019quantifying}&Trust&Quan.&Text&\cmark&\xmark&\cmark&\xmark\\
                                      &Compreh.&&&&&\\
        \midrule                             
        
        %Shin
        ~\cite{shin2021effects}&Trust&Quan.&Text&\xmark&\xmark&\cmark&\xmark\\
        &&&&&&\\
        \midrule
        
        %Spinner et al.
        ~\cite{spinner2019explainer}&Compreh.&Qual.&Image&\xmark&\xmark&\cmark&\xmark\\
        \midrule
        
        %Wang et al.
        ~\cite{wang2019designing}&Trust&Qual.&Tabular&\xmark&\xmark&\cmark&\xmark\\
        &&&(Medical)&&&\\
        \midrule
        
        Our Work&Trust&Quan.&Tabular&\xmark&\xmark&\cmark&\cmark\\
                &Compreh.&Qual.&&&&\\        
        
        \bottomrule 
    \end{tabular}
    }
\end{table}
